# Supplementary material for: High-Dimensional Bayesian Optimization via Tree-Structured Additive Models
Source: arXiv:2012.13088 source file (2020-12-24)
Supplement: Supplementary file 1 [file supplemental.pdf]

# Supplementary Document (Appendix): High-Dimensional Bayesian Optimization via Tree-Structured Additive Models

**AAAI 2021**

**Eric Han,**[1] **Ishank Arora,**[2] **Jonathan Scarlett**[1,3]
[1]School of Computing, National University of Singapore
[2]Indian Institute of Technology (BHU) Varanasi
[3]Department of Mathematics & Institute of Data Science, National University of Singapore
eric_han@nus.edu.sg, ishank.arora.cse14@iitbhu.ac.in, scarlett@comp.nus.edu.sg

## S1 Learning the Kernel Parameters

We consider selecting the kernel parameters by maximizing the marginal likelihood, and specifically adopt a well-established gradient approach. To implement gradient-based methods, we compute the partial derivatives of the log-likelihood with respect to the dimensional hyperparameters $\Theta = \{\theta_i : (\ell_i, \sigma_i)\}_{i=1}^{D}$ as (Williams and Rasmussen 2006):

$$\frac{\partial}{\partial\theta}\rho(Z,\theta) = \frac{1}{2}\operatorname{Tr}\left[(\alpha\alpha^T - K^{-1})\sum_{G\in\mathcal{G}}\left(\frac{\partial\kappa^G}{\partial\theta}\right)\right]. \quad \text{(S1)}$$

The inner partial derivative $\partial\kappa^G/\partial\theta$ depends on the choice of kernel. The partial derivative with respect to each lengthscale $\ell_i$ can be computed directly, and for the kernels we consider, this is facilitated by the availability of closed-form kernel expressions. Following our definition of the scale parameter $\sigma^G = \sqrt{\sum_{i\in G}\sigma_i{}^2}$, the partial derivative with respect to each dimensional scale parameter $\sigma_j$ is

$$\frac{\partial\kappa^G}{\partial\sigma_j} = \frac{\partial\kappa^G}{\partial\sigma^G}\left(\frac{\partial}{\partial\sigma_j}\sqrt{\sum_{i\in G}\sigma_i^2}\right) = \frac{\partial\kappa^G}{\partial\sigma^G}\times\frac{\sigma_j}{\sigma^G}. \quad \text{(S2)}$$

Again, $\partial\kappa^G/\partial\sigma^G$ is computed directly from the closed-form kernel expression. Following common practice (Pedregosa et al. 2011; GPy since 2012), we restrict the optimization of the dimensional parameters to $\ell_j \in \left[10^{-2}, 10^5\right]$ and $\sigma_j \in \left[\sqrt{0.1}, 10^5\right]$, ensuring that the kernel parameters are positive and avoid extreme values that can lead to numerical issues. In addition, we avoid making the lower bound on each $\sigma_j$ too small, accounting for the equivalent effect in the graph learning of not creating an edge between two variables. There exist several gradient-based optimization techniques that can be used, e.g., Limited-Memory Broyden-Fletcher-Goldfarb-Shanno Algorithm (L-BFGS), Truncated Newton algorithm (TNC), and others. We adopt TNC for all experiments except BO-based adversarial attacks, in which we use L-BFGS for consistency with a previous baseline. In addition, we impose limits on the maximum number of function evaluations in terms of the iteration index $t$ according to the following:

$$m(t) = M_0\exp\left(\frac{\log(M_{N_{iter}})}{N_{iter}}\times t\right). \quad \text{(S3)}$$

We found that by increasing the maximum number of function evaluations over iterations, we can get a good trade-off between exploration and exploration, avoiding overfitting of kernel parameters. In (S3), we set $M_0 = 1$ and $M_{N_{iter}} = 2D$.

## S2 Maximization over Discrete Domains

For BO to be effective in high dimensions, the underlying acquisition function needs to be optimized efficiently. In Alg. S1, we present a simplified variant of the algorithm proposed by (Rolland et al. 2018) for generalized additive models. We deal with the optimization of the acquisition function of a given dependency structure $\mathcal{G}$ and discrete domain $\mathcal{X} = \times_{i=1}^{D}\mathcal{X}_i$ with $\mathcal{X}_i = [[a_i, b_i]]$, discretized uniformly with $R$ discrete values between $a_i$ and $b_i$ inclusive. The algorithm uses the message passing technique on a triangulated graph, similar to the efficient maximization of probability in Markov random fields (Wainwright 2015). We will shortly discuss a simplified variant in the case of tree-structured graphs.

Alg. S1 makes use of a junction tree, with each node in the junction tree representing a maximal clique of the triangulated dependency graph. Since we have changed the structure of the dependency graph by triangulation, we need to carefully account for the individual acquisition functions $\phi^G$ (see 4), as they are no longer directly equivalent to the function that we are optimizing on each node of the junction tree. We simplify Rolland *et al.*'s method by excluding the acquisition functions $\phi^G$ that have been previously maximized:

$$\psi^C\left(x^C\right) = \sum_{\forall G\in\mathcal{G}:(\phi^G\notin\Phi\,\bigwedge\,G\subseteq C)}\phi^G\left(x^G\right), \quad \text{(S4)}$$

where $\Phi$ denotes the set of acquisition functions that have been previously maximized. Fig. S1 shows an example.

**Complexity.** Alg. S1 applies to arbitrary graph structures, allowing this technique to be applied to general additive models. The complexity of running the algorithm is exponential in the size of the maximum clique of the triangulated

Copyright © 2021, Association for the Advancement of Artificial Intelligence (www.aaai.org). All rights reserved.

**Algorithm S1:** MSG-PASSING-DISCRETE

Select a node $R$ to root the junction tree
$D_{\text{tree}} \leftarrow$ depth of the rooted tree
Initialize $\Phi \leftarrow \varnothing$
**for** $d = D_{\text{tree}}, \ldots, 1$ **do**
  **for** *every node $C$ at distance $d$ from $R$* **do**
    $C_p = \text{parent}(C)$
    Common variables $I \leftarrow C \cap C_{\text{parent}}$
    Marginal variables $J \leftarrow C \backslash C_{\text{parent}}$
    **for** $x^I \in \mathcal{X}^I$ **do**
      $M_{C \to C_p}\left[x^I\right] = \max_{x^J \in \mathcal{X}^J} \psi^C\left(x^I, x^J\right) + \sum_{C_c \in \text{children}(C)} M_{C_c \to C}\left[x^{C \cap C_c}\right]$
    Update $\Phi$ to include all $\phi^G$ that were optimized in $\psi^C$
**return** $\max_{x^R \in \mathcal{X}^R} \psi^R\left(x^R\right) + \sum_{C_c \in \text{children}(R)} M_{C_c \to R}\left[x^{R \cap C_c}\right]$

graph (Rolland et al. 2018). Hence, the algorithm can benefit from choosing a triangulation that minimizes the size of the maximal clique (Arnborg, Corneil, and Proskurowski 1987; Cano and Moral 1994). In Tree, the dependency structure is a tree. As a result, there are no cycles, and there is no need to triangulate the tree $\mathcal{G}$. Moreover, the function of $\psi^C$ can be simplified to $\psi^C = \phi^C$. Hence, the complexity of the maximization is reduced to quadratic in $R$.

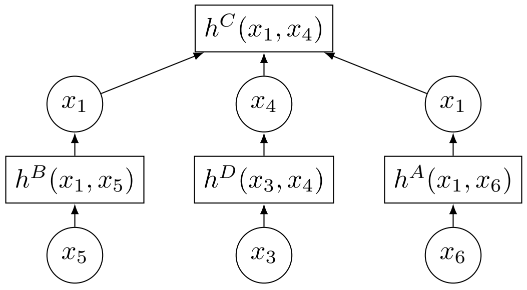


Figure S1: Illustration of the optimization of the acquisition function on the graph $\mathcal{G}$ shown in Fig. 1. First, the leaves of the junction tree perform partial maximization of the functions $f^B$, $f^D$, and $f^A$ over their respective variables $x_4$, $x_2$ and $x_5$. The result of the partial maximization is a 'conditional' maximization over the other variables. These 'conditional' maximizations are passed as messages to the nodes above. In this manner, the messages are passed until the root node, and the correct answer is returned.

## S3 Implementation Details

We implemented all algorithms in Python 3.8.3. The Python environments are managed using Conda, and experiments are managed using MLflow (Zaharia et al. 2018). The specific hardware used is not crucial, as we ensure consistent runs across different hardware via the use of Conda and MLflow.

Both Graph Overlap and Graph No-Overlap are reimplemented using the original implementations and the details from their publications (Rolland et al. 2018; Kandasamy, Schneider, and Póczos 2015).

For LineBO algorithms, we use the original author's implementation.[1] The REMBO and InterleavedREMBO implementations are also based on the implementation found in LineBO's repository. We additionally consider the heuristic NelderMead algorithm (Nelder and Mead 1965), which is provided by SciPy, as in LineBO's repository. Implementation of the algorithms used in the BO-Based Adversarial Attack experiments are from the original author's repository.[2]

## S4 Further Experimental Details and Results

The existing algorithms that we use in our experiments, along with their parameters, are summarized in Table S1. We note that for parameters unique to LineBO, we have used the recommended parameters as stated in (Kirschner et al. 2019),

| Method | Unique parameter values |
|---|---|
| DescentLineBO<br>RandomLineBO<br>CoordinateLineBO | As per hartmann6.yaml[3] |
| REMBO | Embedded Dimension $= \sqrt{D}$ |
| InterleavedREMBO | Interleaved Runs = 4 |
| NelderMead | Contraction Factor $= 0.3$<br>Initial Stepsize $= 0.1$<br>Restart Threshold $= 0.001$ |
| Graph No-Overlap<br>Graph Overlap | Max Clique Size$= D$<br>N/A |
| ADDGP-BO<br>GP-BO | As per defaults in repository[2] |

Table S1: State-of-the-art methods' parameters values

[1]https://github.com/jkirschner42/LineBO
[2]https://github.com/rubinxin/BayesOpt_Attack

| Type | Name | Dim. | No. of Exps. |
|---|---|---|---|
| Add. GP Fns. | Grid-3×3 | 9 | 250 |
| | Star-10 | 10 | 250 |
| | Partition-12 | 12 | 250 |
| | Star-25 | 25 | 250 |
| | Ancestry-132 | 132 | 125 |
| Add. GP Fns. (Scalability) | Grid-2×2 | 4 | 125 |
| | Grid-3×3 | 9 | 125 |
| | Grid-4×4 | 16 | 125 |
| | Grid-5×5 | 25 | 100 |
| | Grid-6×6 | 36 | 100 |
| | Grid-7×7 | 49 | 50 |
| | Grid-8×8 | 64 | 50 |
| | Grid-9×9 | 81 | 50 |
| | Grid-10×10 | 100 | 25 |
| | Grid-11×11 | 121 | 25 |
| | Grid-12×12 | 144 | 25 |
| | Grid-13×13 | 169 | 25 |
| | Grid-14×14 | 196 | 25 |
| | Grid-15×15 | 225 | 25 |
| Non-GP Fns. | Camelback2 | 2 | 150 |
| | Hartmann6 | 6 | 150 |
| | Camelback2+10Aux | 12 | 150 |
| | Hartmann6+14Aux | 20 | 150 |
| | Rosenbrock20 | 20 | 150 |
| | Stybtang250 | 250 | 150 |
| NAS | naval | 9 | 100 |
| | parkinsons | | 100 |
| | protein | | 100 |
| | slice | | 100 |
| Lpsolve | misc05inf | | 150 |
| | mtest4ma | 74 | 150 |
| | qiu | | 150 |
| BA | MNIST | 196 | 1800 |

Table S2: Summary of both Synthetic (top) and Real (bottom) functions used in our experiments; by type, dimensionality.

specifically the parameters found in their Hartmann6 experiments.[3]

A summary of the functions that were used in our experiments is given in Table S2. We ran the functions in the 'Additive GP Functions' experiments over both continuous and discrete domains, investigating Tree's performance. The rest of the functions were run over continuous domains.

## S4.1 Additive GP Functions

In addition to the observations made in the main document, Tree's efficiency is also demonstrated for both discrete and continuous functions – see Fig. S3-S4. We see that Tree is able to learn a tree structure that performs well while being cost-efficient, even when the hypothesis that Tree considers

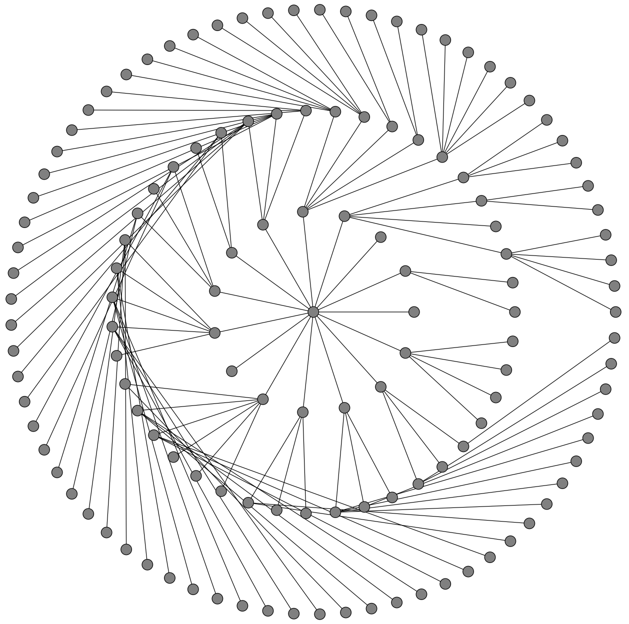

Figure S2: Ancestry-132 Dependency Graph Structure.

is not realizable in both Grid-3×3 and Partition-12. In the case of Partition-12, Tree's graph learning is not realizable, whereas both Graph No-Overlap and Graph Overlap are realizable. The results for Partition-12 lends further support to the discussion in Sec. 4.3 on Grid-3×3, Tree remains competitive in terms of the optimization performance despite poorer graph learning. Most surprisingly, Tree is sometimes able to outperform Oracle; see Fig. S3g and Fig. S3j. To understand this, recall from Sec. 4.1 that we limited the number of individual acquisition function evaluations to 1000. For tree structures, we are dealing with functions of at most two variables, whereas this limitation in evaluations has the greatest impact on graphs whose triangulated versions have larger cliques. In the present example, the true graph provided for Oracle contains cliques of size at least 3 after triangulation. These results suggest that even when the hypothesis is not realizable, the performance penalty for Tree is minor. That is, the lack of model richness is compensated for by faster model selection and the ability to optimize the acquisition function accurately.

In addition, we ran experiments on Ancestry-132, a 132-dimensional family tree of (Nicolas Kruchten 2015), shown in Fig. S2. The graph was obtained from the original author's repository and converted to an equivalent representation for use in our codebase.[4] We used the graph structure in the same way as any of the synthetic dependency graphs structures, which we specified in Sec. 4.3. We note that for higher dimensions, $\mathrm{F_1score}$ in Fig. S5b may potentially improve by increasing the number of graphs $S$ sampled in Alg. 3;

[3] In the repository of (Kirschner et al. 2019) – https://github.com/jkirschner42/LineBO/blob/master/config/hartmann6.yaml

[4] https://raw.githubusercontent.com/nicolaskruchten/genealogy/master/family.json

we have adopted the same choice across all experiments for consistency.

## S4.2 Non-GP Functions

**Synthetic Functions.** Camelback2 is a commonly used BO benchmark function with two dimensions that has two global minima with the same value of $-1.0316$ (Eggensperger et al. 2013). Hartmann6 (6D) is defined as

$$f(x) = -\sum_{i=1}^{4} \alpha_i \exp\left(-\sum_{j=1}^{6} A_{ij}\left(x_j - P_{ij}\right)^2\right), \quad \text{(S5)}$$

and has seven minima – six local and one global (Eggensperger et al. 2013). We use implementations from HPOlib2, letting $\alpha, A$ and $P$ be as defined in (Eggensperger et al. 2013). Rosenbrock20 (20D) is a synthetic function that have a single global optima at $x = (1.0, \ldots, 1.0)$ with value of 0. Rosenbrock20 is challenging to optimize, as the values returned by the function have a wide range even when using a small domain of $[0, 1]$. The Styblinski-Tang function, Stybtang250 (250D):

$$f(x) = \frac{1}{2}\sum_{i=1}^{250}(x_i^4 - 16x_i^2 + 5x_i), \quad \text{(S6)}$$

has a global minimum of approximately $-39.16599 \times 250$ at $x = (-2.9, \ldots, -2.9)$. We restrict the domain of the function to $[-4, 4]^{250}$. Similar to Rosenbrock20, the values returned by Stybtang250 has a wide range.

From Fig. S6a-S6f, we observe that Tree consistently performs well across these synthetic functions. In contrast, the LineBO algorithms perform better on certain functions than others, and can face certain limitations. For instance, from Fig. S6e, we see that LineBO algorithms can incur higher regret to perform when the range of the function is large, which applies to both Rosenbrock20 and Stybtang250.

**Linear Programming Solver.** Here, we include further lpsolve experiments to supplement those in the main text. REMBO and its interleaved variant are effective in some cases (e.g., Fig. S7a), but are slow to converge in others (e.g., Fig. S7a, Fig. S7b). In contrast, Tree performs well across all three datasets.

**NAS Benchmarks.** We run experiments on the NAS-Bench-101 (NAS) dataset (Ying et al. 2019; Klein and Hutter 2019). This dataset serves as a convenient hyperparameter benchmark that allows us to quickly run hyperparameter optimization over a fully connected neural network. Traditionally, when we run hyperparameter optimization over a neural network, it would be slow, as training and testing a neural network would take substantial time. This benchmark pre-computes the results for all possible 62208 configurations (from 9 hyperparameters) defined in (Ying et al. 2019; Klein and Hutter 2019). Consequently, we have access to $f_{\max}$. We ran the experiments as described in (Klein and Hutter 2019), across all four NAS benchmarks (see Table S2).

The results from the NAS benchmarks suggest that most functions in this dataset have little additive structure. We can observe this from the lack of significant difference between the graph-based algorithms across the NAS-naval, NAS-parkinsons and NAS-slice as shown in Fig. S8. There is a small performance edge that Tree achieves over the other algorithms in NAS-protein shown in Fig. S8c. The performance edge is gained efficiently, requiring lower cost when compared with the rest of the algorithms. Overall, these experiments suggest that Tree does not break down in datasets with little or no additive structure while retaining efficiency.

**BO-Based Adversarial Attack.** BO has recently been applied to *targeted* adversarial black-box attacks on neural networks. In particular, (Ru et al. 2020) proposed an approach based on the non-overlapping additive model from (Kandasamy, Schneider, and Póczos 2015). Their method achieves comparable success rates with fewer queries than certain state-of-the-art black-box attack methods for attacks on convolutional neural network (CNN) models. We adopt the same black-box function as (Ru et al. 2020), in which the input is an image perturbation and the output is the classification accuracy.

In this experiment, we adapt Tree in an analogous manner to (Ru et al. 2020) in order to perform adversarial black-box attacks on the CNN models. To maintain a fair comparison, we adopted the same experimental choices and parameters as (Ru et al. 2020) wherever possible, in particular using the Matérn-$5/2$ kernel, applying L-BFGS for kernel parameter optimization, performing graph and parameter learning according to the same regularly-spaced intervals (length 40 and 5 respectively), and using $N_{\text{init}} = 50$ initial random points.

The CNN models that we attack are also the same as (Tu et al. 2019; Alzantot et al. 2019; Ru et al. 2020). The image classifiers for the dataset MNIST (99.5% Accuracy) is taken from the author's repository. Using the same reduction technique and dimensionality as (Ru et al. 2020; Tu et al. 2019), we perform the search on a reduced image dimension of $14 \times 14 \times 1$ for MNIST (196D). For the attack, we randomly select 50 correctly-classified images; then, for each image, we perform the attack for all target labels except the true label. We record the Attack Success Rate (ASR) (i.e., the proportion of times the attack succeeds in making the classifier output the target label, averaged across 450 runs) against the number of iterations. We used process time from Python's standard library[5], recording the total of both system and user process-wide CPU time. Considering that we executed the experiments over a hetrogenous cluster (randomly distributed) and other experimental considerations, this metric allows us to glean a rough measure of the algorithm's efficiency.

We compare Tree to the implementations available in (Ru et al. 2020)'s repository. We note that the additive BO implementation (ADDGP-BO) is different from our implementation of Graph No-Overlap. In particular, they select the graph according the highest likelihood among a number of randomly-generated graphs, whereas we adopt the Gibbs sampling approach of (Wang et al. 2017; Rolland et al. 2018).

We focus on comparing against ADDGP-BO, as it was the

[5]https://docs.python.org/3/library/time.html#time.process time

best overall method reported in (Ru et al. 2020). The results are presented in Fig. S9.[6] We see in Fig. S9a that Tree is able to attack MNIST (196D) CNN model with a comparable success rate as ADDGP-BO, but with significantly reduced process time. The process time is lowest for GP-BO (an GP-UCB based baseline without additive structure, available in the repository of (Ru et al. 2020)), but at the cost of a significantly worse ASR.

## References (Appendix only)


Alzantot, M.; Sharma, Y.; Chakraborty, S.; Zhang, H.; Hsieh, C.-J.; and Srivastava, M. B. 2019. Genattack: Practical black-box attacks with gradient-free optimization. In *Proceedings of the Genetic and Evolutionary Computation Conference*, 1111–1119.

Arnborg, S.; Corneil, D. G.; and Proskurowski, A. 1987. Complexity of finding embeddings in a $k$-tree. *SIAM Journal on Algebraic Discrete Methods* 8(2):277–284.

Cano, A., and Moral, S. 1994. Heuristic algorithms for the triangulation of graphs. In *International Conference on Information Processing and Management of Uncertainty in Knowledge-Based Systems*, 98–107. Springer.

Eggensperger, K.; Feurer, M.; Hutter, F.; Bergstra, J.; Snoek, J.; Hoos, H.; and Leyton-Brown, K. 2013. Towards an empirical foundation for assessing Bayesian optimization of hyperparameters. In *NIPS Workshop on Bayesian Optimization in Theory and Practice*.

GPy. since 2012. GPy: A Gaussian process framework in python. http://github.com/SheffieldML/GPy.

Kandasamy, K.; Schneider, J.; and Póczos, B. 2015. High dimensional Bayesian optimisation and bandits via additive models. In *Int. Conf. Mach. Learn. (ICML)*, 295–304.

Kirschner, J.; Mutny, M.; Hiller, N.; Ischebeck, R.; and Krause, A. 2019. Adaptive and safe Bayesian optimization in high dimensions via one-dimensional subspaces. In *Int. Conf. Mach. Learn. (ICML)*, 3429–3438.

Klein, A., and Hutter, F. 2019. Tabular benchmarks for joint architecture and hyperparameter optimization. *arXiv preprint arXiv:1905.04970*.

Nelder, J. A., and Mead, R. 1965. A simplex method for function minimization. *The Computer Journal* 7(4):308–313.

Nicolas Kruchten. 2015. Visualizing Family Trees. http://nicolas.kruchten.com/content/2015/08/family-trees/. Accessed: 2020-06-01.

Pedregosa, F.; Varoquaux, G.; Gramfort, A.; Michel, V.; Thirion, B.; Grisel, O.; Blondel, M.; Prettenhofer, P.; Weiss, R.; Dubourg, V.; Vanderplas, J.; Passos, A.; Cournapeau, D.; Brucher, M.; Perrot, M.; and Duchesnay, E. 2011. Scikit-learn: Machine learning in Python. *Journal of Machine Learning Research* 12:2825–2830.

Rolland, P.; Scarlett, J.; Bogunovic, I.; and Cevher, V. 2018. High-dimensional Bayesian optimization via additive models with overlapping groups. In *Int. Conf. Art. Intel. Stats. (AISTATS)*, 298–307.

Ru, B.; Cobb, A.; Blaas, A.; and Gal, Y. 2020. BayesOpt Adversarial Attack. In *Proc. of the International Conference on Learning Representations*.

Tu, C.-C.; Ting, P.; Chen, P.-Y.; Liu, S.; Zhang, H.; Yi, J.; Hsieh, C.-J.; and Cheng, S.-M. 2019. Autozoom: Autoencoder-based zeroth order optimization method for attacking black-box neural networks. In *AAAI Conf. on Art. Intel.*, volume 33, 742–749.


[6] Attacks that took at least three times longer than 99% of the runs were marked as unsuccessful.


Wainwright, M. J. 2015. Graphical models and message-passing algorithms: Some introductory lectures. In *Mathematical Foundations of Complex Networked Information Systems*. Springer. 51–108.

Wang, Z.; Li, C.; Jegelka, S.; and Kohli, P. 2017. Batched high-dimensional Bayesian optimization via structural kernel learning. In *Int. Conf. Mach. Learn. (ICML)*, 3656–3664. JMLR. org.

Williams, C. K., and Rasmussen, C. E. 2006. *Gaussian processes for machine learning*, volume 2. MIT press Cambridge, MA.

Ying, C.; Klein, A.; Christiansen, E.; Real, E.; Murphy, K.; and Hutter, F. 2019. NAS-Bench-101: Towards reproducible neural architecture search. In *Int. Conf. Mach. Learn. (ICML)*, 7105–7114.

Zaharia, M.; Chen, A.; Davidson, A.; Ghodsi, A.; Hong, S. A.; Konwinski, A.; Murching, S.; Nykodym, T.; Ogilvie, P.; Parkhe, M.; et al. 2018. Accelerating the Machine Learning Lifecycle with MLflow. *IEEE Data Eng. Bull.* 41(4):39–45.

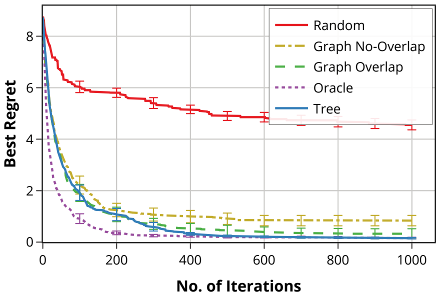


(a) Star-10 (Discrete) Performance

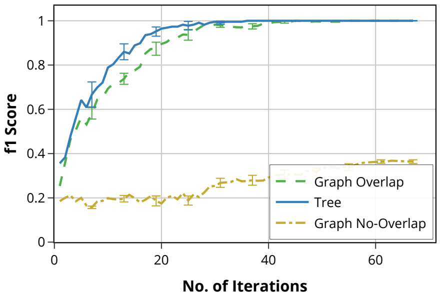


(b) Star-10 (Discrete) $F_1$score

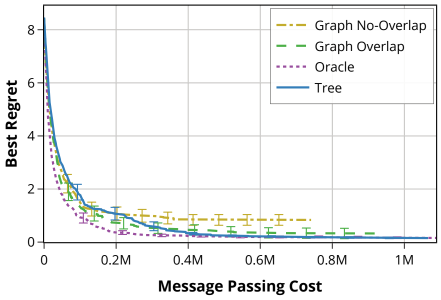


(c) Star-10 (Discrete) Cost

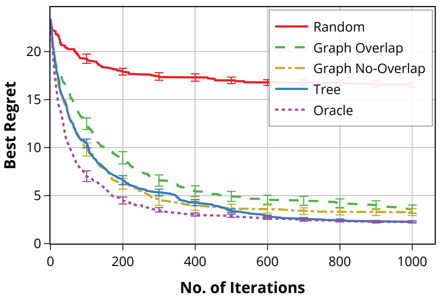


(d) Star-25 (Discrete) Performance

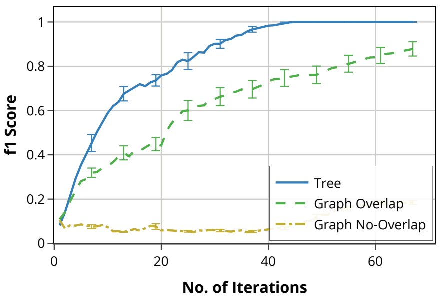


(e) Star-25 (Discrete) $F_1$score

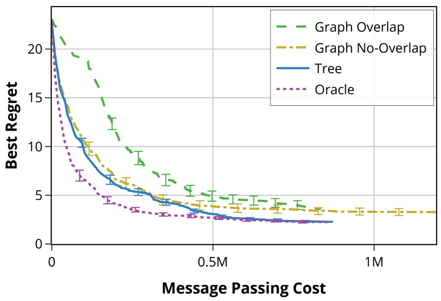


(f) Star-25 (Discrete) Cost

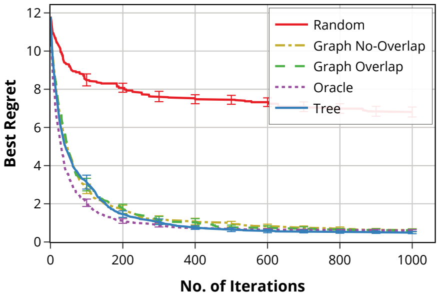


(g) Partition-12 (Discrete) Performance

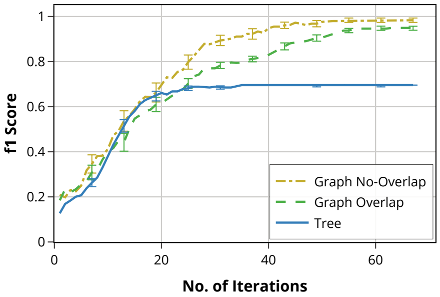


(h) Partition-12 (Discrete) $F_1$score

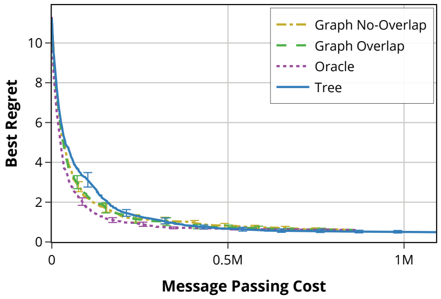


(i) Partition-12 (Discrete) Cost

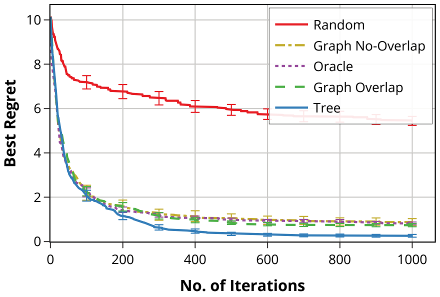


(j) Grid-3×3 (Discrete) Performance

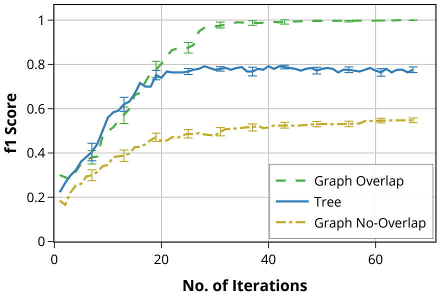


(k) Grid-3×3 (Discrete) $F_1$score

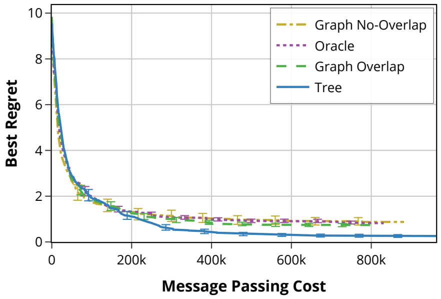


(l) Grid-3×3 (Discrete) Cost

Figure S3: Results for synthetic additive functions on discrete domains.

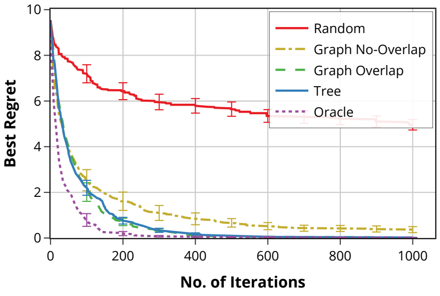


(a) Star-10 (Continuous) Performance

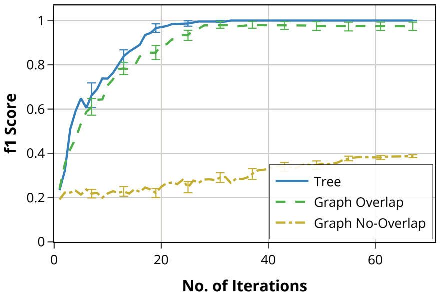


(b) Star-10 (Continuous) $F_1$score

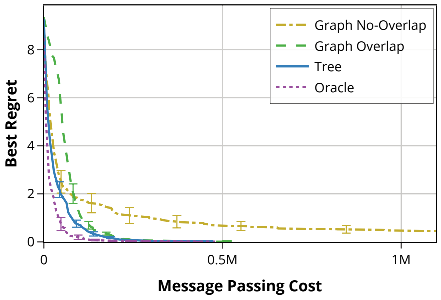


(c) Star-10 (Continuous) Cost

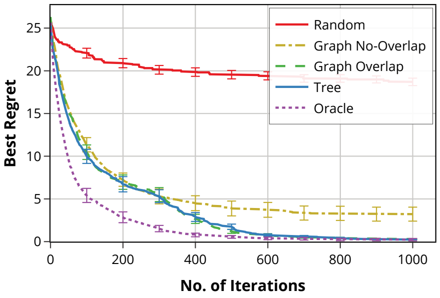


(d) Star-25 (Continuous) Performance

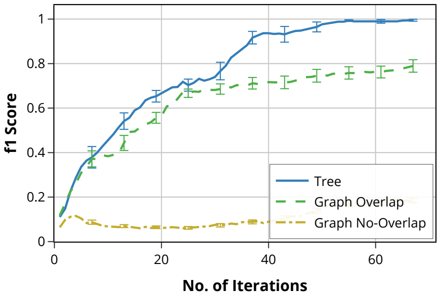


(e) Star-25 (Continuous) $F_1$score

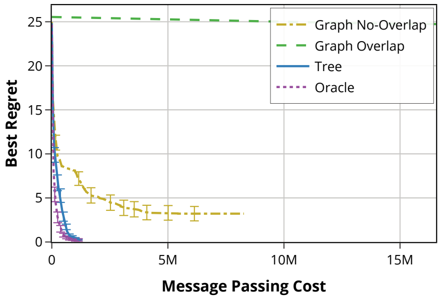


(f) Star-25 (Continuous) Cost

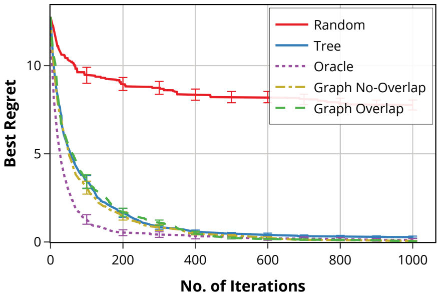


(g) Partition-12 (Continuous) Performance

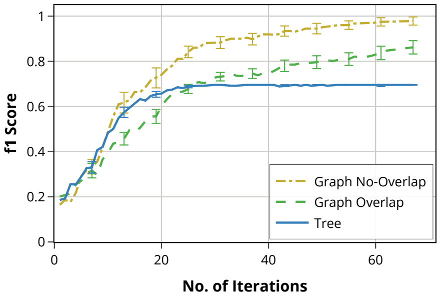


(h) Partition-12 (Continuous) $F_1$score

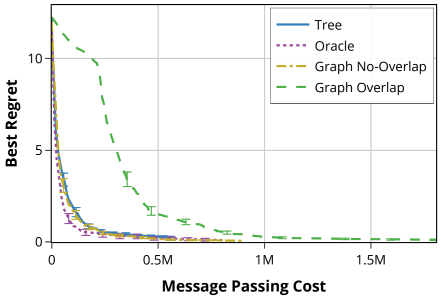


(i) Partition-12 (Continuous) Cost

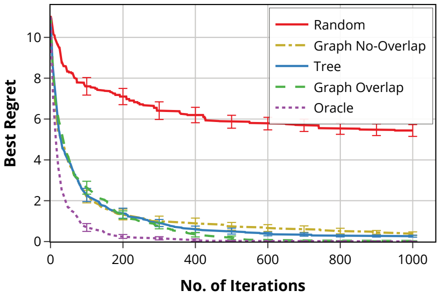


(j) Grid-3×3 (Continuous) Performance

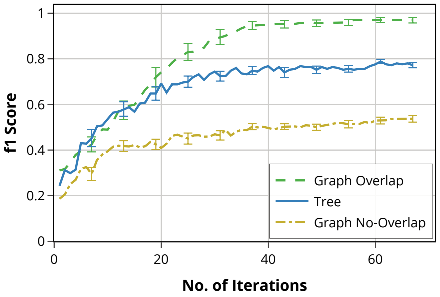


(k) Grid-3×3 (Continuous) $F_1$score

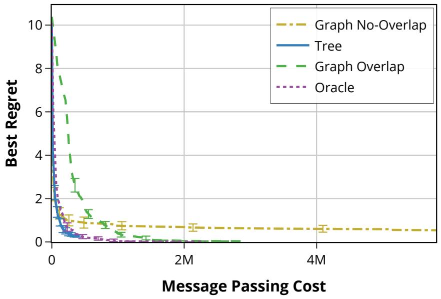


(l) Grid-3×3 (Continuous) Cost

Figure S4: Results of synthetic additive functions on continuous domains.

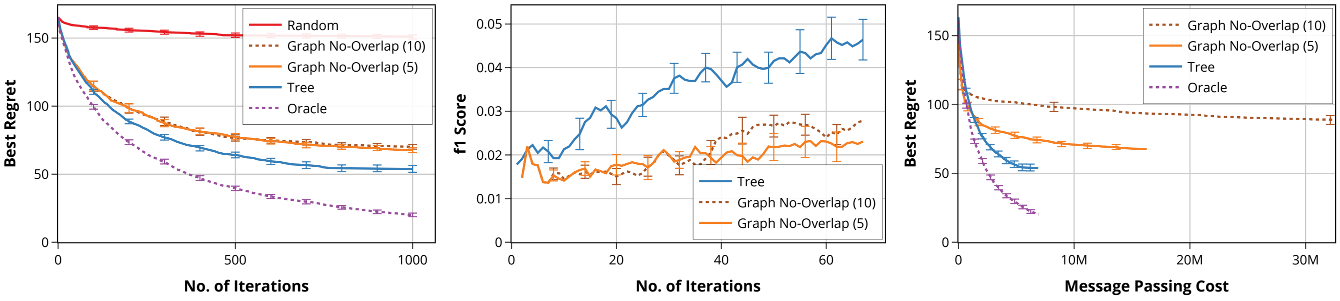


(a) Ancestry-132 (Continuous) Performance (b) Ancestry-132 (Continuous) $F_1$score (c) Ancestry-132 (Continuous) Cost

Figure S5: Results for the Ancestry-132 graph.

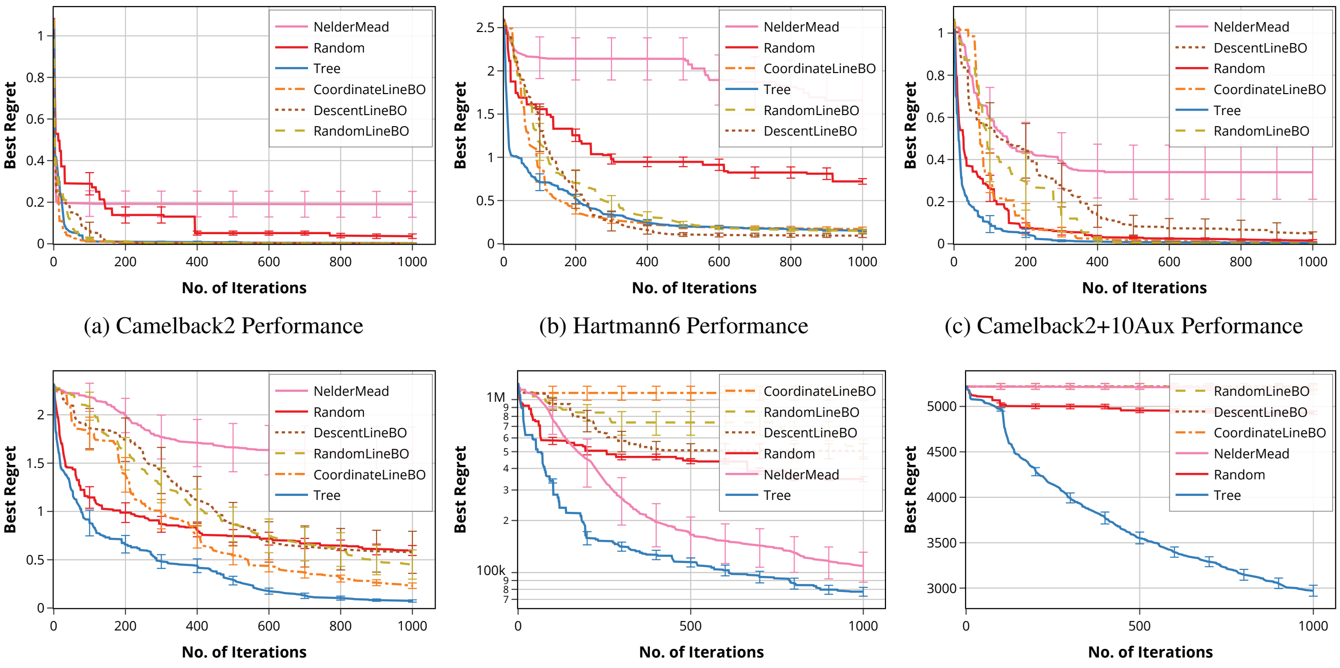


(a) Camelback2 Performance (b) Hartmann6 Performance (c) Camelback2+10Aux Performance

(d) Hartmann6+14Aux Performance (e) Rosenbrock20 Performance (f) Stybtang250 Performance

Figure S6: Results for non-GP synthetic functions.

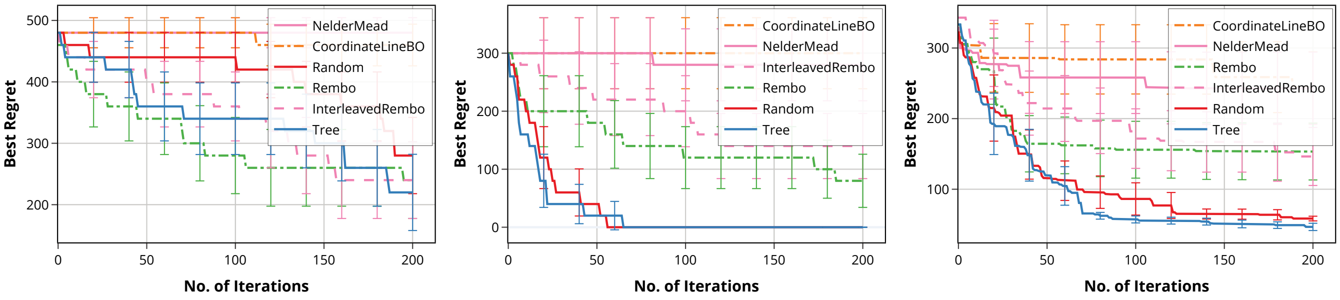


(a) Lpsolve-misc05inf Performance (b) Lpsolve-mtest4ma Performance (c) Lpsolve-qiu Performance

Figure S7: Results for Lpsolve hyperparameter tuning.

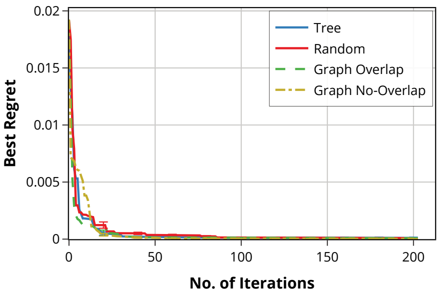


(a) NAS-naval Performance

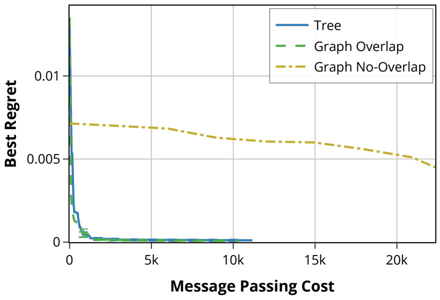


(b) NAS-naval Cost

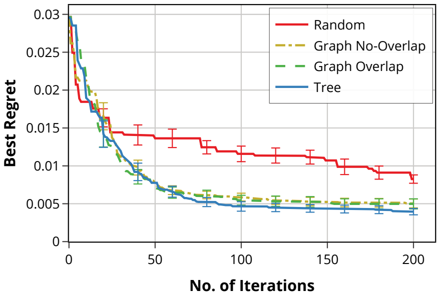


(c) NAS-parkinsons Performance

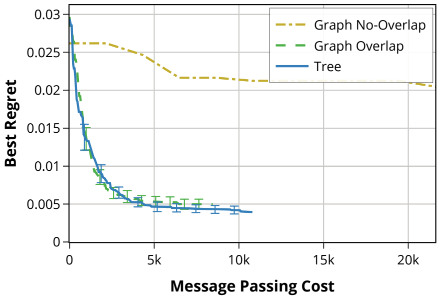


(d) NAS-parkinsons Cost

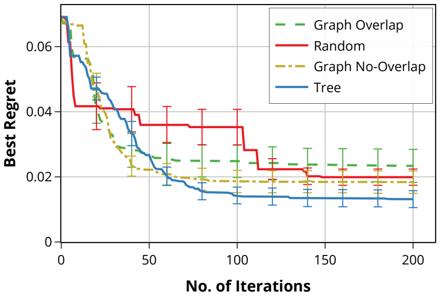


(e) NAS-protein Performance

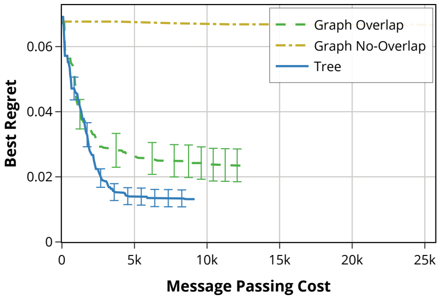


(f) NAS-protein Cost

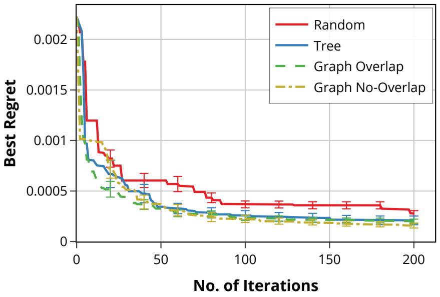


(g) NAS-slice Performance

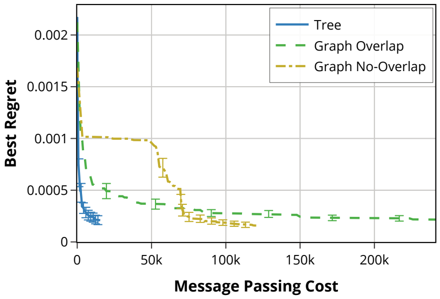


(h) NAS-slice Cost

Figure S8: Results for NAS-Bench-101 datasets.

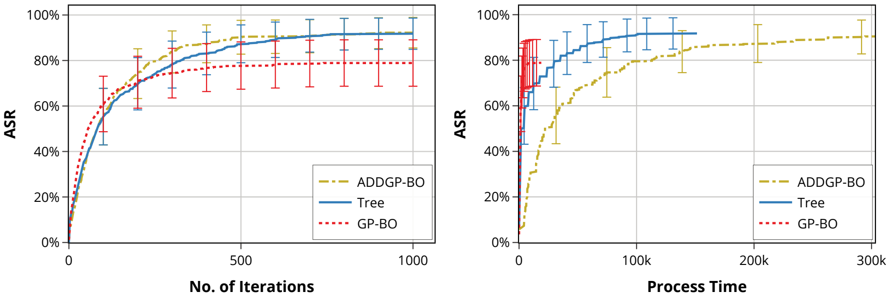


(a) BA-MNIST Performance (b) BA-MNIST Cost

Figure S9: Results for BO-based adversarial attacks.
